# Supplementary material for: Magnetic bound states embedded in tantalum superconducting thin films
Source: arXiv:2412.15903 source file (2025-04-12)

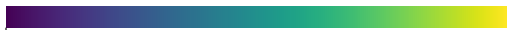

.....

.....









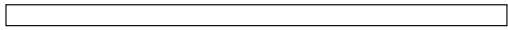

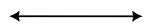

-

|

|

|

|

|

|

|









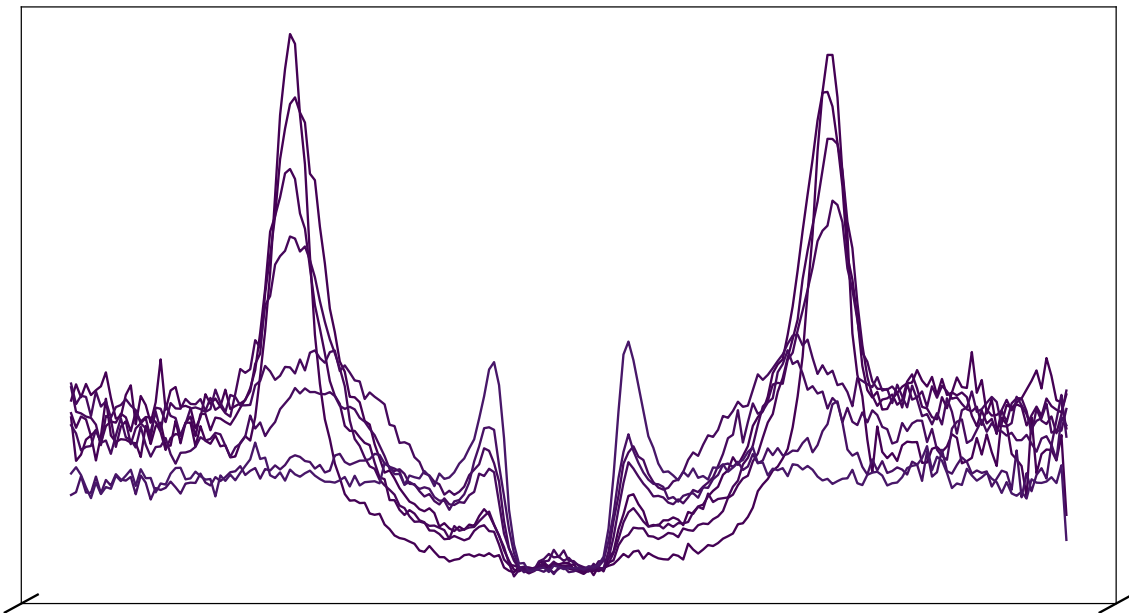





















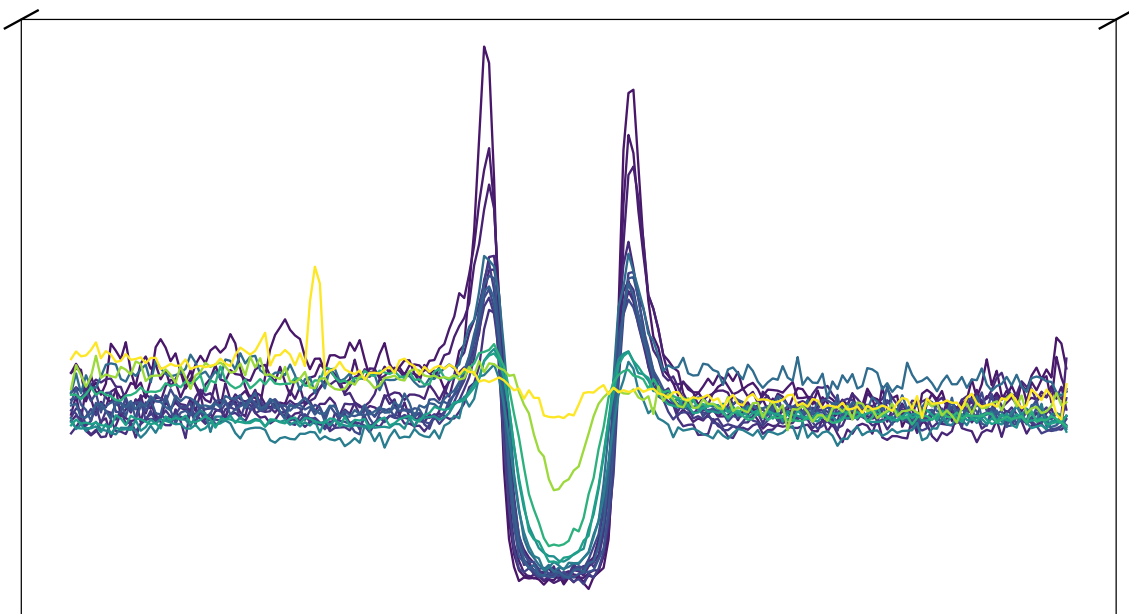

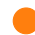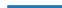

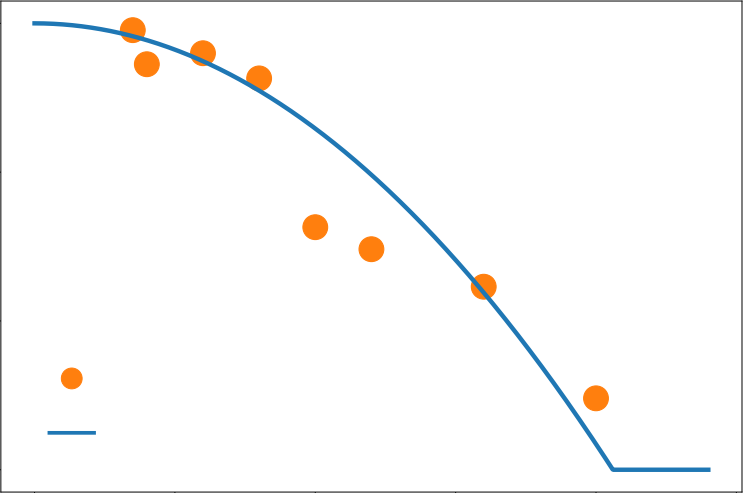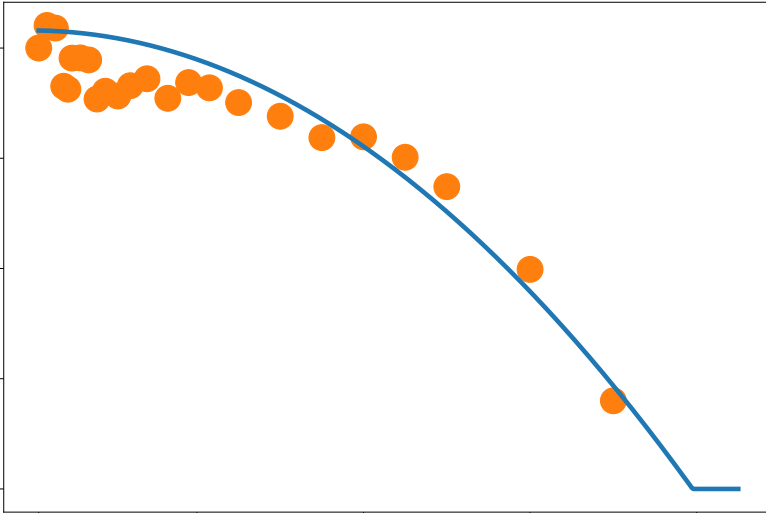

Supplement: Supplementary file 1 [file supplement_latex.pdf]
